# Supplementary material for: Firth's logistic regression with rare events: accurate effect estimates AND predictions?
Source: arXiv:2101.07620 ancillary file (2021-01-19)
Supplement: Supplementary file 1 [file Supplement.pdf]

# Supplementary material for "Firth's logistic regression with rare events: accurate effect estimates AND predictions?" by Rainer Puhr et al.

Supplementary table 1: Mean bias and RMSE ($\times 10000$) of predicted probabilities $\hat{\pi}_i$, mean and standard deviation ($\times 100$) of calibration slopes, for the simulation scenarios with coefficients of mixed signs omitted in Table 2.

| N | $\pi$ | Method | Predictions | | | | | | Calibration slope | | | |
|---|---|---|---|---|---|---|---|---|---|---|---|---|
| | | | **Bias** ($\times 10000$) | | | **RMSE** ($\times 10000$) | | | **Mean** ($\times 100$) | | **SD** ($\times 100$) | |
| | | | $a$ | | | $a$ | | | $a$ | | $a$ | |
| | | | 0 | 0.5 | 1 | 0 | 0.5 | 1 | 0.5 | 1 | 0.5 | 1 |
| 1400 | 0.02 | ML | -3 | -2 | -2 | 133 | 165 | 231 | 48 | 85 | 17 | 20 |
| | | WF | 5 | 5 | 4 | 137 | 169 | 232 | 47 | 84 | 16 | 19 |
| | | FL | 34 | 34 | 29 | 155 | 186 | 238 | 44 | 80 | 14 | 17 |
| | | FLIC | -3 | -2 | -2 | 130 | 159 | 218 | 51 | 90 | 17 | 21 |
| | | FLAC | -3 | -2 | -2 | 119 | 147 | 215 | 56 | 97 | 20 | 25 |
| | | LF | -3 | -2 | -2 | 130 | 161 | 224 | 50 | 87 | 17 | 21 |
| | | CP | -2 | -1 | -2 | 125 | 156 | 219 | 52 | 90 | 18 | 22 |
| | | AU | -3 | -2 | -2 | 133 | 167 | 234 | 48 | 84 | 17 | 20 |
| | | AB | 71 | 69 | 60 | 186 | 214 | 253 | 40 | 76 | 11 | 14 |
| | | RR | -3 | -2 | -2 | 57 | 116 | 213 | 134 | 116 | 80 | 51 |
| | 0.05 | ML | -2 | -1 | -2 | 199 | 232 | 278 | 73 | 93 | 17 | 13 |
| | | WF | 5 | 5 | 4 | 201 | 233 | 278 | 72 | 93 | 17 | 13 |
| | | FL | 33 | 31 | 26 | 210 | 240 | 279 | 70 | 92 | 16 | 12 |
| | | FLIC | -2 | -1 | -2 | 196 | 227 | 271 | 74 | 95 | 17 | 13 |
| | | FLAC | -2 | -1 | -2 | 190 | 222 | 270 | 77 | 97 | 18 | 14 |
| | | LF | -2 | -1 | -2 | 197 | 230 | 274 | 73 | 93 | 17 | 13 |
| | | CP | -1 | -1 | -1 | 194 | 227 | 271 | 75 | 95 | 17 | 13 |
| | | AU | -2 | -1 | -2 | 199 | 233 | 279 | 73 | 92 | 17 | 13 |
| | | AB | 67 | 63 | 53 | 228 | 253 | 283 | 67 | 91 | 14 | 12 |
| | | RR | -2 | -1 | -2 | 112 | 200 | 269 | 115 | 102 | 42 | 17 |
| | 0.10 | ML | -1 | -2 | -2 | 270 | 294 | 316 | 83 | 95 | 13 | 9 |
| | | WF | 5 | 4 | 3 | 271 | 294 | 315 | 83 | 95 | 13 | 9 |
| | | FL | 29 | 26 | 21 | 275 | 295 | 315 | 83 | 95 | 13 | 9 |
| | | FLIC | -1 | -2 | -2 | 267 | 289 | 311 | 84 | 97 | 13 | 9 |
| | | FLAC | -1 | -2 | -2 | 263 | 288 | 311 | 86 | 97 | 14 | 9 |
| | | LF | -1 | -2 | -2 | 268 | 292 | 314 | 84 | 95 | 14 | 9 |
| | | CP | -1 | -1 | -2 | 266 | 290 | 312 | 85 | 96 | 14 | 9 |
| | | AU | -1 | -2 | -2 | 270 | 294 | 317 | 83 | 95 | 13 | 9 |
| | | AB | 60 | 54 | 45 | 284 | 300 | 316 | 82 | 96 | 13 | 8 |
| | | RR | -1 | -2 | -2 | 183 | 276 | 310 | 105 | 99 | 24 | 10 |
| 3000 | 0.10 | ML | -1 | 0 | 0 | 183 | 202 | 214 | 91 | 98 | 11 | 6 |
| | | WF | 2 | 3 | 2 | 184 | 202 | 214 | 91 | 98 | 11 | 6 |
| | | FL | 14 | 13 | 11 | 185 | 203 | 214 | 91 | 98 | 11 | 6 |
| | | FLIC | -1 | 0 | 0 | 183 | 200 | 212 | 92 | 98 | 11 | 6 |
| | | FLAC | -1 | 0 | 0 | 181 | 200 | 212 | 93 | 99 | 11 | 6 |
| | | LF | -1 | 0 | 0 | 183 | 201 | 213 | 92 | 98 | 11 | 6 |
| | | CP | -1 | 0 | 0 | 182 | 201 | 212 | 92 | 98 | 11 | 6 |
| | | AU | -1 | 0 | 0 | 183 | 202 | 214 | 91 | 98 | 11 | 6 |
| | | AB | 28 | 26 | 21 | 188 | 204 | 214 | 90 | 98 | 10 | 6 |
| | | RR | -1 | 0 | 0 | 147 | 197 | 212 | 101 | 100 | 15 | 6 |

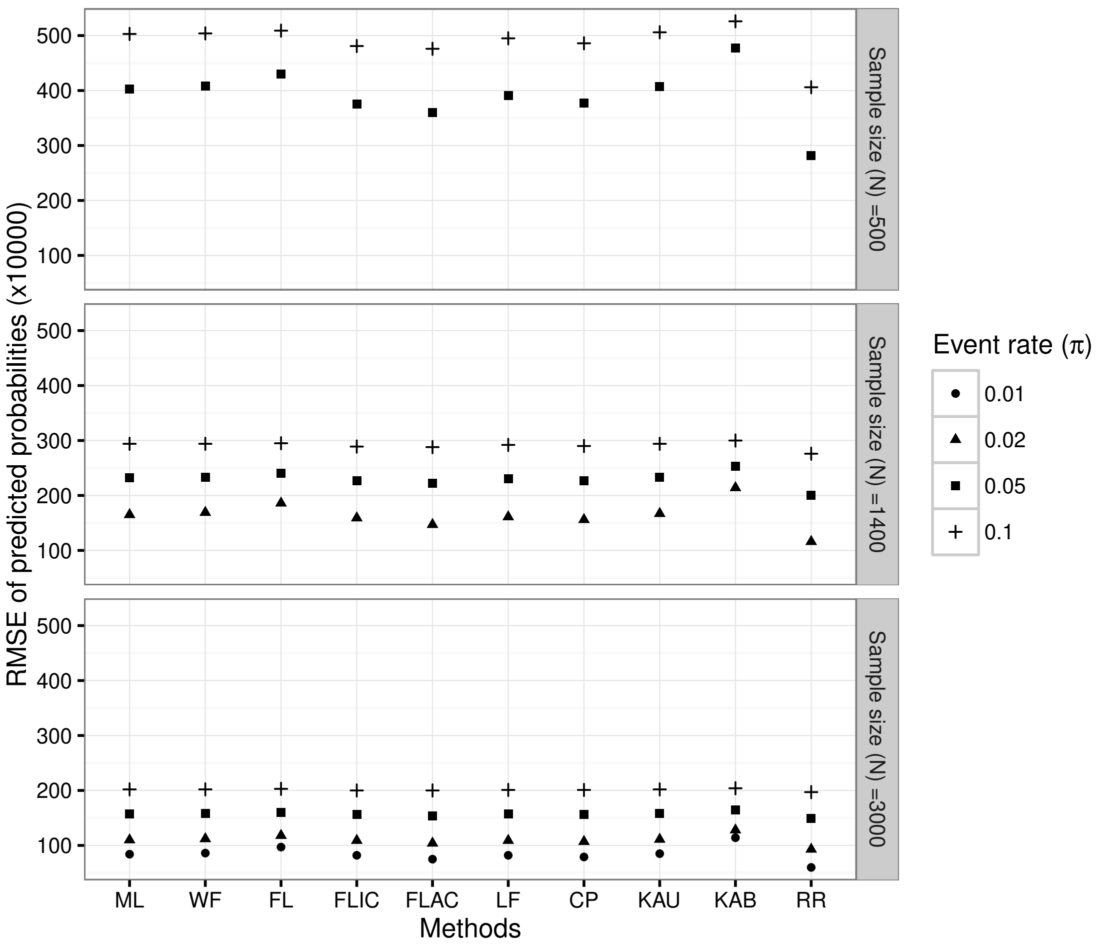


Supplementary figure 1: RMSE of predicted probabilities ($\times 10000$) for scenarios with small effect sizes ($a = 0.5$) and with coefficients of mixed signs, see also Table 2 and Supplementary table 1.

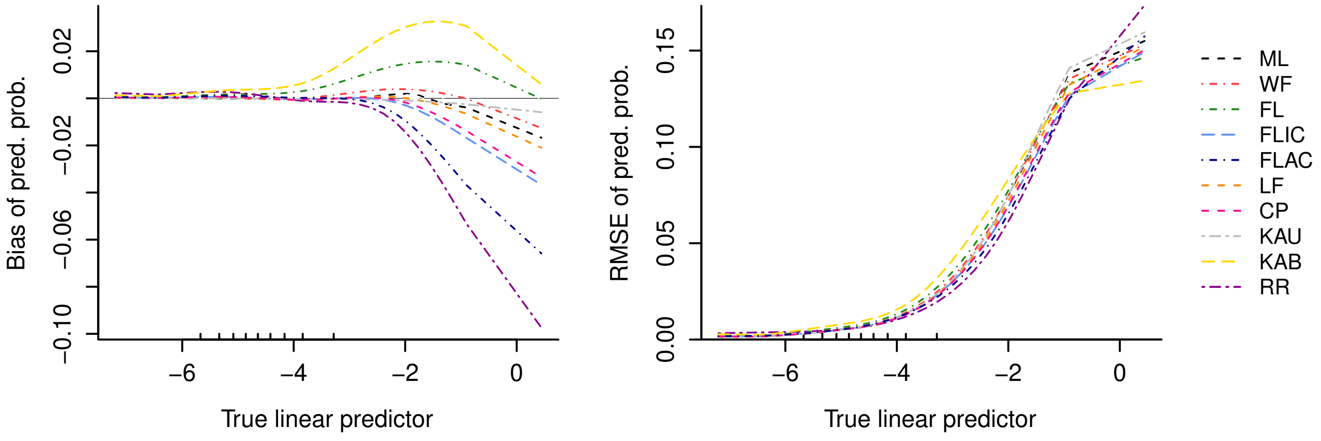


Supplementary figure 2: Bias and RMSE of predicted probabilities by true linear predictor, exemplarily for the scenario $N = 1400$, $\bar{y} = 0.02$, large effect size ($a = 1$) and coefficients of mixed signs. For the calculation of bias and RMSE, the predicted probabilities were splitted into 30 groups using adequate quantiles of the true linear predictor. Cubic smoothing splines were then fitted to the derived bias and RMSE values in the 30 groups. Upward directed ticks on the x-axis mark the deciles of the true linear predictor. See Figure 1 for a scaled version of this plot.

Supplementary table 2: Mean and standard deviation of c-indices ($\times 1000$) with regard to a newly drawn outcome, for selected scenarios with coefficients of mixed signs. The "optimal value" was calculated as the c-index for the predicted probabilities of the true model.

| **N** | $\pi$ | **Method** | **c-statistic** | | | |
|---|---|---|---|---|---|---|
| | | | **Mean** $\times 1000$ | | **SD** $\times 1000$ | |
| | | | $a$ | | $a$ | |
| | | | 0.5 | 1 | 0.5 | 1 |
| 500 | 0.05 | optimal | 650 | 790 | 59 | 49 |
| | | ML | 602 | 753 | 60 | 57 |
| | | WF | 602 | 754 | 60 | 57 |
| | | FL/FLIC | 604 | 754 | 60 | 56 |
| | | FLAC | 601 | 754 | 60 | 57 |
| | | LF | 602 | 754 | 60 | 57 |
| | | CP | 602 | 755 | 60 | 57 |
| | | AU | 600 | 751 | 60 | 58 |
| | | AB | 606 | 756 | 60 | 56 |
| | | RR | 605 | 754 | 60 | 57 |
| | 0.10 | optimal | 646 | 774 | 43 | 36 |
| | | ML | 609 | 752 | 47 | 40 |
| | | WF | 609 | 752 | 47 | 40 |
| | | FL/FLIC | 610 | 752 | 46 | 40 |
| | | FLAC | 608 | 752 | 47 | 40 |
| | | LF | 609 | 752 | 47 | 40 |
| | | CP | 609 | 752 | 47 | 40 |
| | | AU | 608 | 751 | 47 | 40 |
| | | AB | 611 | 752 | 46 | 40 |
| | | RR | 609 | 751 | 45 | 40 |
| 1400 | 0.05 | optimal | 648 | 790 | 34 | 30 |
| | | ML | 622 | 776 | 38 | 33 |
| | | WF | 622 | 776 | 38 | 33 |
| | | FL/FLIC | 622 | 776 | 38 | 33 |
| | | FLAC | 621 | 776 | 38 | 33 |
| | | LF | 622 | 776 | 38 | 33 |
| | | CP | 622 | 776 | 38 | 33 |
| | | AU | 621 | 775 | 38 | 33 |
| | | AB | 623 | 776 | 38 | 33 |
| | | RR | 622 | 775 | 38 | 33 |
| 3000 | 0.01 | optimal | 651 | 813 | 52 | 45 |
| | | ML | 605 | 788 | 55 | 49 |
| | | WF | 605 | 789 | 55 | 49 |
| | | FL/FLIC | 607 | 789 | 55 | 49 |
| | | FLAC | 604 | 789 | 55 | 49 |
| | | LF | 605 | 789 | 55 | 49 |
| | | CP | 605 | 790 | 55 | 49 |
| | | AU | 603 | 787 | 55 | 50 |
| | | AB | 609 | 790 | 55 | 49 |
| | | RR | 611 | 790 | 55 | 49 |
| | 0.05 | optimal | 648 | 789 | 24 | 20 |
| | | ML | 634 | 782 | 26 | 21 |
| | | WF | 634 | 782 | 26 | 21 |
| | | FL/FLIC | 634 | 782 | 26 | 21 |
| | | FLAC | 634 | 782 | 26 | 21 |
| | | LF | 634 | 782 | 26 | 21 |
| | | CP | 634 | 782 | 26 | 21 |
| | | AU | 634 | 782 | 26 | 21 |
| | | AB | 634 | 782 | 26 | 21 |
| | | RR | 633 | 782 | 26 | 21 |

Supplementary table 3: Bias and RMSE ($\times 100$) of linear predictors $x_i\beta$, for selected simulation scenarios with coefficients of mixed signs.

| **N** | $\pi$ | **Method** | **Bias** ($\times 100$) | | | **RMSE** ($\times 100$) | | |
|---|---|---|---|---|---|---|---|---|
| | | | $a$ | | | $a$ | | |
| | | | 0 | 0.5 | 1 | 0 | 0.5 | 1 |
| 500 | 0.05 | ML | -25 | -24 | -31 | 85 | 82 | 94 |
| | | WF | -20 | -19 | -24 | 82 | 79 | 89 |
| | | FL | -2 | -2 | -1 | 72 | 71 | 77 |
| | | FLIC | -21 | -20 | -19 | 76 | 75 | 81 |
| | | FLAC | -20 | -17 | -14 | 73 | 71 | 78 |
| | | LF | -23 | -22 | -25 | 82 | 78 | 85 |
| | | CP | -21 | -19 | -19 | 76 | 74 | 80 |
| | | RR | -5 | 1 | 2 | 34 | 50 | 71 |
| | 0.10 | ML | -11 | -11 | -14 | 55 | 55 | 62 |
| | | WF | -9 | -9 | -11 | 54 | 54 | 60 |
| | | FL | -1 | -1 | -1 | 51 | 51 | 56 |
| | | FLIC | -10 | -10 | -9 | 52 | 52 | 57 |
| | | FLAC | -10 | -9 | -8 | 51 | 51 | 56 |
| | | LF | -11 | -11 | -12 | 54 | 54 | 59 |
| | | CP | -10 | -10 | -9 | 53 | 53 | 57 |
| | | RR | -3 | 1 | 0 | 27 | 41 | 54 |
| 1400 | 0.02 | ML | -23 | -22 | -27 | 75 | 73 | 82 |
| | | WF | -19 | -18 | -21 | 73 | 71 | 79 |
| | | FL | -3 | -2 | -1 | 66 | 65 | 70 |
| | | FLIC | -21 | -20 | -18 | 70 | 69 | 73 |
| | | FLAC | -19 | -15 | -12 | 66 | 65 | 70 |
| | | LF | -22 | -20 | -22 | 73 | 70 | 76 |
| | | CP | -20 | -18 | -18 | 69 | 67 | 73 |
| | | RR | -6 | 1 | 3 | 30 | 46 | 65 |
| | 0.05 | ML | -8 | -8 | -10 | 43 | 43 | 47 |
| | | WF | -7 | -6 | -8 | 43 | 42 | 46 |
| | | FL | -1 | 0 | -1 | 41 | 41 | 44 |
| | | FLIC | -8 | -7 | -7 | 42 | 41 | 45 |
| | | FLAC | -7 | -6 | -6 | 41 | 41 | 44 |
| | | LF | -8 | -8 | -9 | 43 | 42 | 46 |
| | | CP | -8 | -7 | -7 | 42 | 41 | 45 |
| | | RR | -3 | 2 | 0 | 24 | 35 | 43 |
| | 0.10 | ML | -4 | -4 | -5 | 31 | 30 | 34 |
| | | WF | -3 | -3 | -4 | 30 | 30 | 34 |
| | | FL | 0 | 0 | -1 | 30 | 29 | 33 |
| | | FLIC | -4 | -3 | -4 | 30 | 30 | 33 |
| | | FLAC | -4 | -3 | -3 | 30 | 29 | 33 |
| | | LF | -4 | -4 | -5 | 30 | 30 | 33 |
| | | CP | -4 | -3 | -4 | 30 | 30 | 33 |
| | | RR | -2 | 1 | -1 | 20 | 27 | 32 |
| 3000 | 0.01 | ML | -20 | -19 | -23 | 72 | 69 | 78 |
| | | WF | -16 | -15 | -18 | 70 | 67 | 75 |
| | | FL | -2 | -1 | 0 | 64 | 62 | 68 |
| | | FLIC | -19 | -18 | -17 | 68 | 66 | 71 |
| | | FLAC | -17 | -13 | -9 | 64 | 62 | 67 |
| | | LF | -19 | -17 | -19 | 70 | 66 | 72 |
| | | CP | -18 | -15 | -15 | 66 | 64 | 69 |
| | | RR | -4 | 3 | 4 | 30 | 46 | 63 |
| | 0.05 | ML | -4 | -3 | -4 | 29 | 28 | 31 |
| | | WF | -3 | -3 | -3 | 29 | 28 | 31 |
| | | FL | 0 | 0 | 0 | 28 | 28 | 30 |
| | | FLIC | -4 | -3 | -3 | 28 | 28 | 30 |
| | | FLAC | -4 | -3 | -2 | 28 | 28 | 30 |
| | | LF | -4 | -3 | -4 | 29 | 28 | 31 |
| | | CP | -4 | -3 | -3 | 28 | 28 | 30 |
| | | RR | -2 | 1 | 0 | 20 | 26 | 30 |

Supplementary table 4: Absolute bias and RMSE ($\times 1000$) of standardized coefficients, averaged over all explanatory variables (except for the intercept), for the simulation scenarios with coefficients of mixed signs omitted in Table 3.

| **N** | $\pi$ | **Method** | **Bias** ($\times 1000$) | | | **RMSE** ($\times 1000$) | | |
|---|---|---|---|---|---|---|---|---|
| | | | $a$ | | | $a$ | | |
| | | | 0 | 0.5 | 1 | 0 | 0.5 | 1 |
| 1400 | 0.02 | ML | 19 | 11 | 19 | 244 | 235 | 246 |
| | | WF | 16 | 9 | 15 | 241 | 232 | 242 |
| | | FL/FLIC | 6 | 5 | 4 | 230 | 221 | 229 |
| | | FLAC | 15 | 14 | 14 | 215 | 211 | 222 |
| | | LF | 18 | 9 | 7 | 235 | 224 | 231 |
| | | CP | 16 | 14 | 20 | 221 | 215 | 222 |
| | | RR | 2 | 107 | 114 | 73 | 155 | 219 |
| | 0.05 | ML | 7 | 5 | 12 | 149 | 144 | 153 |
| | | WF | 7 | 5 | 10 | 149 | 144 | 152 |
| | | FL/FLIC | 4 | 4 | 4 | 145 | 141 | 148 |
| | | FLAC | 7 | 7 | 7 | 142 | 138 | 147 |
| | | LF | 7 | 5 | 7 | 147 | 142 | 150 |
| | | CP | 7 | 7 | 10 | 144 | 140 | 147 |
| | | RR | 2 | 77 | 53 | 63 | 125 | 150 |
| | 0.10 | ML | 3 | 3 | 10 | 107 | 104 | 115 |
| | | WF | 3 | 3 | 8 | 107 | 104 | 114 |
| | | FL/FLIC | 2 | 3 | 3 | 106 | 102 | 112 |
| | | FLAC | 3 | 4 | 3 | 104 | 102 | 112 |
| | | LF | 3 | 3 | 6 | 107 | 103 | 113 |
| | | CP | 3 | 4 | 4 | 105 | 102 | 112 |
| | | RR | 1 | 53 | 26 | 60 | 100 | 113 |
| 3000 | 0.10 | ML | 2 | 3 | 4 | 72 | 72 | 76 |
| | | WF | 2 | 3 | 4 | 72 | 71 | 76 |
| | | FL/FLIC | 2 | 2 | 2 | 72 | 71 | 75 |
| | | FLAC | 2 | 2 | 2 | 72 | 71 | 75 |
| | | LF | 2 | 3 | 3 | 72 | 71 | 76 |
| | | CP | 2 | 2 | 2 | 72 | 71 | 75 |
| | | RR | 2 | 25 | 12 | 53 | 71 | 75 |

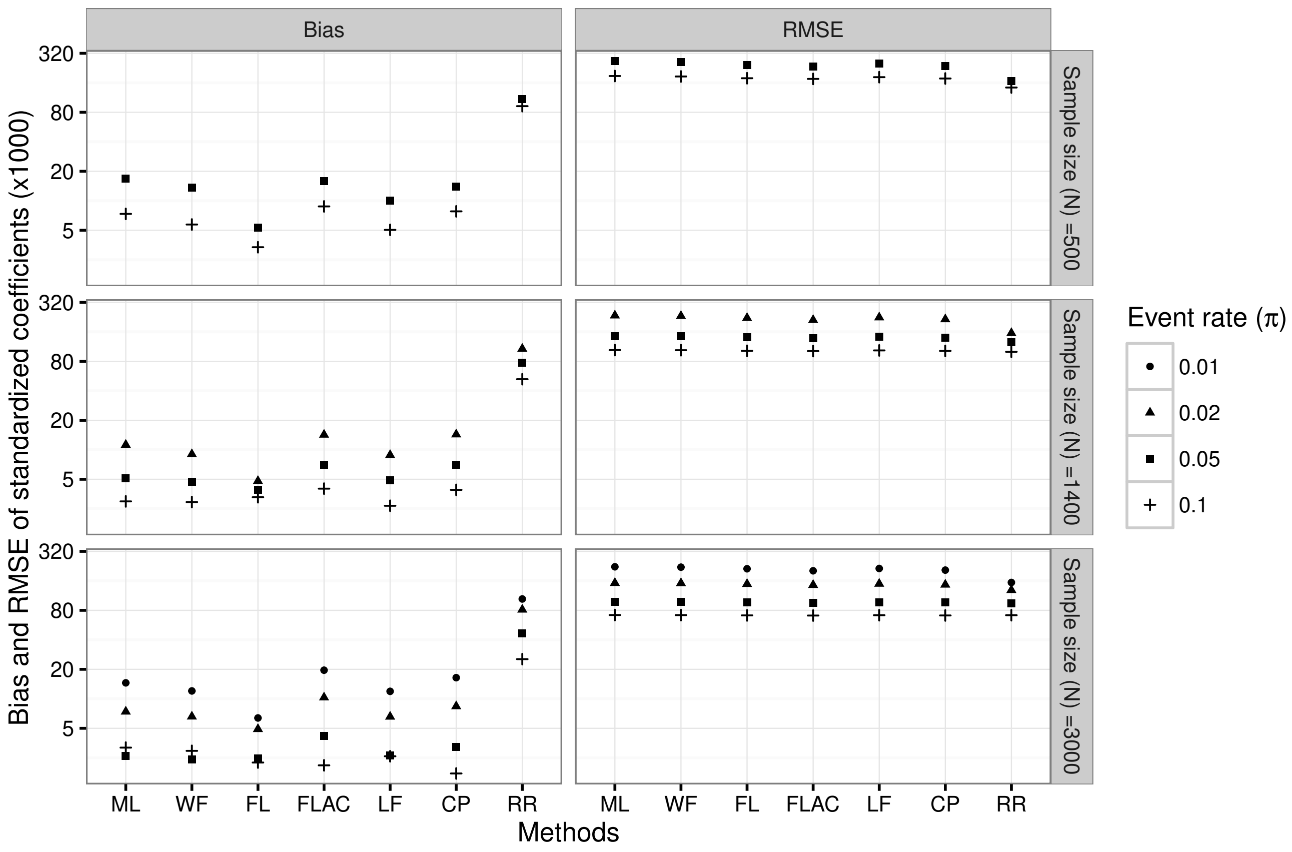


Supplementary figure 3: Absolute bias and RMSE ($\times 1000$) of standardized coefficients on logarithmic scale, averaged over all explanatory variables (omitting the intercept), for scenarios with small effect sizes ($a = 0.5$) and with coefficients of mixed signs, see also Table 3 and Supplementary table 4.

Supplementary table 5: Coverage, power ($\times 1000$) and length ($\times 100$) of approximate Wald-type, bootstrap and jackknife 95% confidence intervals in Firth estimation with intercept correction of the intercept $\beta_0$, for the simulation scenarios with non-zero coefficients of mixed signs and sample size smaller than 3000.

| **N** | $\pi$ | **Method** | **Coverage** ($\times 1000$) | | **Power**($\times 1000$) | | **Length**($\times 100$) | |
|---|---|---|---|---|---|---|---|---|
| | | | $a$ | | $a$ | | $a$ | |
| | | | 0.5 | 1 | 0.5 | 1 | 0.5 | 1 |
| 500 | 0,05 | approximate | 958 | 974 | 297 | 347 | 974 | 1047 |
| | | bootstrap | 957 | 973 | 290 | 309 | 997 | 1116 |
| | | jackknife | 955 | 965 | 305 | 335 | 978 | 1078 |
| | 0,10 | approximate | 953 | 953 | 308 | 383 | 699 | 748 |
| | | bootstrap | 954 | 960 | 308 | 368 | 709 | 774 |
| | | jackknife | 950 | 959 | 320 | 379 | 701 | 762 |
| 1400 | 0,02 | approximate | 965 | 957 | 542 | 614 | 874 | 934 |
| | | bootstrap | 957 | 953 | 534 | 593 | 877 | 954 |
| | | jackknife | 956 | 947 | 534 | 598 | 879 | 947 |
| | 0,05 | approximate | 946 | 947 | 685 | 762 | 560 | 598 |
| | | bootstrap | 943 | 955 | 686 | 759 | 561 | 606 |
| | | jackknife | 946 | 952 | 682 | 760 | 562 | 603 |
| | 0,10 | approximate | 958 | 946 | 743 | 854 | 408 | 438 |
| | | bootstrap | 964 | 949 | 737 | 854 | 411 | 442 |
| | | jackknife | 956 | 950 | 732 | 851 | 409 | 439 |

Supplementary table 6: Coverage, power and standardized length ($\times 1000$) of $95\%$-confidence intervals, averaged over all explanatory variables (omitting the intercept), for selected simulation scenarios with coefficients of mixed signs.

| **N** | $\pi$ | **Method** | **Coverage** ($\times 1000$) | | | **Length** ($\times 1000$) | | | **Power** ($\times 1000$) | |
|---|---|---|---|---|---|---|---|---|---|---|
| | | | $a$ | | | $a$ | | | $a$ | |
| | | | 0 | 0.5 | 1 | 0 | 0.5 | 1 | 0.5 | 1 |
| 500 | 0.05 | ML | 952 | 951 | 953 | 1016 | 987 | 1059 | 133 | 326 |
| | | WF | 945 | 944 | 944 | 1019 | 990 | 1061 | 136 | 341 |
| | | FL/FLIC | 952 | 950 | 954 | 986 | 957 | 1019 | 128 | 321 |
| | | FLAC | 956 | 953 | 950 | 945 | 926 | 979 | 114 | 323 |
| | | LF | 949 | 948 | 951 | 1004 | 971 | 1032 | 128 | 327 |
| | | CP | 959 | 958 | 959 | 954 | 930 | 980 | 116 | 295 |
| | | RR | 996 | 912 | 863 | 462 | 536 | 772 | 45 | 238 |
| | 0.10 | ML | 949 | 946 | 946 | 715 | 707 | 763 | 197 | 477 |
| | | WF | 945 | 943 | 943 | 716 | 708 | 763 | 199 | 488 |
| | | FL/FLIC | 949 | 948 | 948 | 702 | 694 | 745 | 192 | 472 |
| | | FLAC | 952 | 947 | 946 | 690 | 684 | 731 | 184 | 476 |
| | | LF | 946 | 944 | 946 | 711 | 702 | 753 | 195 | 478 |
| | | CP | 954 | 952 | 950 | 693 | 686 | 732 | 183 | 447 |
| | | RR | 995 | 896 | 900 | 401 | 462 | 645 | 91 | 378 |
| 1400 | 0.02 | ML | 953 | 951 | 952 | 925 | 888 | 933 | 147 | 367 |
| | | WF | 948 | 947 | 946 | 928 | 891 | 935 | 148 | 384 |
| | | FL/FLIC | 951 | 950 | 951 | 909 | 872 | 910 | 147 | 367 |
| | | FLAC | 960 | 955 | 950 | 871 | 845 | 880 | 129 | 369 |
| | | LF | 951 | 950 | 950 | 916 | 877 | 915 | 142 | 372 |
| | | CP | 960 | 958 | 955 | 879 | 847 | 879 | 132 | 340 |
| | | RR | 996 | 909 | 873 | 443 | 509 | 714 | 57 | 275 |
| | 0.05 | ML | 948 | 950 | 952 | 576 | 560 | 596 | 268 | 610 |
| | | WF | 946 | 947 | 950 | 576 | 561 | 596 | 269 | 618 |
| | | FL/FLIC | 948 | 950 | 952 | 571 | 555 | 589 | 267 | 608 |
| | | FLAC | 951 | 952 | 952 | 562 | 549 | 581 | 258 | 613 |
| | | LF | 947 | 949 | 951 | 574 | 558 | 591 | 266 | 613 |
| | | CP | 952 | 952 | 953 | 564 | 550 | 581 | 259 | 590 |
| | | RR | 996 | 894 | 922 | 364 | 409 | 536 | 164 | 524 |
| | 0.10 | ML | 949 | 952 | 947 | 414 | 409 | 440 | 414 | 796 |
| | | WF | 948 | 951 | 945 | 414 | 409 | 440 | 416 | 800 |
| | | FL/FLIC | 950 | 953 | 948 | 412 | 407 | 436 | 413 | 794 |
| | | FLAC | 951 | 953 | 948 | 409 | 405 | 433 | 409 | 797 |
| | | LF | 949 | 952 | 947 | 413 | 408 | 438 | 414 | 798 |
| | | CP | 951 | 954 | 950 | 410 | 405 | 434 | 405 | 785 |
| | | RR | 989 | 903 | 933 | 307 | 340 | 417 | 307 | 751 |
| 3000 | 0.01 | ML | 951 | 953 | 951 | 877 | 839 | 866 | 153 | 401 |
| | | WF | 948 | 947 | 945 | 881 | 842 | 869 | 158 | 417 |
| | | FL/FLIC | 949 | 950 | 949 | 866 | 828 | 850 | 155 | 405 |
| | | FLAC | 958 | 956 | 951 | 831 | 803 | 826 | 138 | 402 |
| | | LF | 950 | 950 | 949 | 870 | 830 | 851 | 151 | 406 |
| | | CP | 958 | 958 | 955 | 838 | 804 | 823 | 140 | 373 |
| | | RR | 996 | 903 | 881 | 437 | 496 | 685 | 65 | 310 |
| | 0.02 | ML | 947 | 952 | 949 | 611 | 588 | 611 | 249 | 574 |
| | | WF | 947 | 949 | 947 | 612 | 589 | 612 | 251 | 585 |
| | | FL/FLIC | 947 | 951 | 949 | 607 | 584 | 605 | 250 | 574 |
| | | FLAC | 952 | 954 | 950 | 595 | 575 | 597 | 236 | 578 |
| | | LF | 948 | 950 | 949 | 609 | 585 | 607 | 246 | 579 |
| | | CP | 951 | 956 | 953 | 598 | 576 | 596 | 237 | 549 |
| | | RR | 996 | 898 | 908 | 375 | 418 | 544 | 146 | 487 |
| | 0.05 | ML | 948 | 948 | 950 | 388 | 377 | 399 | 455 | 836 |
| | | WF | 947 | 947 | 949 | 388 | 377 | 399 | 459 | 839 |
| | | FL/FLIC | 948 | 948 | 951 | 387 | 376 | 397 | 455 | 836 |
| | | FLAC | 949 | 950 | 950 | 384 | 374 | 395 | 453 | 838 |
| | | LF | 947 | 948 | 950 | 387 | 376 | 398 | 457 | 838 |
| | | CP | 950 | 950 | 950 | 385 | 374 | 395 | 447 | 829 |
| | | RR | 987 | 903 | 937 | 296 | 322 | 382 | 354 | 798 |
